# Supplementary material for: Scalable probes of measurement-induced criticality
Source: arXiv:1910.00020 source file (2020-06-10)
Supplement: Supplementary file 1 [file LocalProbe_supp.pdf]

# Supplemental Material: Scalable probes of measurement-induced criticality

## I. DECODING LIGHT CONE

In this section, we present numerical data on the decoding light cone for a single-reference qubit that is locally entangled with an initially volume-law entangled state. We consider two boundary conditions. In Fig. S1(a), we run the circuit at a fixed measurement rate in the volume-law phase until saturation ($t_0 = 4L$), which takes time $\sim L$ [1, 2]. We then measure one qubit, entangle it with the reference, and evolve the system. We find a nearly identical emergent light cone in the purification dynamics of this single reference qubit as we found in the main text for the same conditions starting from a product state ($t_0 = 0$).

In Fig. S1(b), we consider an initial state which is a pseudorandom stabilizer state at $t_0 = 4L$, which is obtained by running the circuit without measurements. We find a similar decoding light cone in the future evolution with measurements. We remark that if the reference starts in a pseudorandom state together with system, then there is no similar light cone observed in the data (not shown). Instead, the measurement events that purify the reference qubit are distributed uniformly randomly throughout the system.

The emergence of this light cone is potentially surprising because strict causality can be violated in these models [3]. As a result, any light cone that emerges is statistical in nature. We leave a full exploration of these issues for future work, but note that the behavior observed here is consistent with another probe of information spreading that uses a single-reference qubit, which was introduced in our recent work [4]. In that approach, we define a light cone by the minimal region over which the system has maximal mutual information with the reference qubit, which remains well-defined to arbitrarily late times in the volume-law phase.

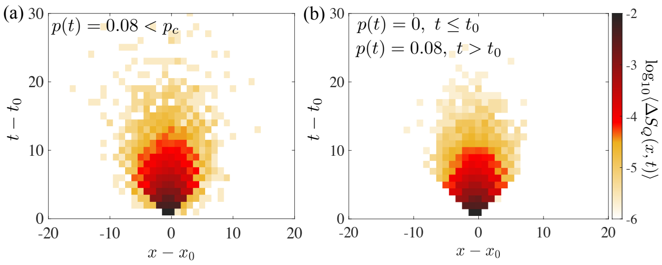


FIG. S1: Decoding light cone starting from volume-law entangled states. At time $t_0 = 4L$ (we took $L = 64$), a qubit in the system is measured and entangled with a reference qubit. In (a) we took a constant value of $p = 0.08 < p_c \approx 0.16$ for all times. In (b) we performed a quench in $p$ from 0 for $t \le t_0$ to $p = 0.08$ for $t > t_0$. Thus, the initial state is a quasirandom stabilizer state.

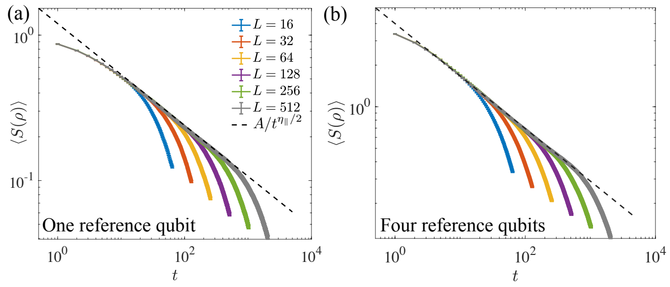


FIG. S2: Purification dynamics of one (a) and four (b) reference qubits at $p = 0.1596 \approx p_c$ starting from a product initial state, periodic boundary conditions, and the reference qubits maximally entangled with a contiguous region. From (a/b) we obtain an estimate $\eta_\parallel = 0.70(2)/0.76(2)$ that lies in the systematic uncertainty interval obtained from the mutual information probes described in the main text.

## II. SURFACE EXPONENT

In this section, we estimate the surface exponent using an alternative numerical method compared to the main text. In particular, we consider the purification dynamics of a finite number of reference qubits at $p_c$ maximally entangled with the system. Following the appearance of this work, Li, Chen, Ludwig and Fisher pointed out that, in 1+1 dimensions, there are advantages to considering the entropy of the reference system to probe $\eta_\parallel$ (instead of the mutual information of two reference qubits) because it maps to a less complicated boundary operator in the underlying conformal field theory [3]. In addition, Li *et al.* suggested that, in stabilizer circuits, it might be advantageous to consider the purification dynamics of several reference qubits instead of just one. The reduced density matrix for a stabilizer state on one qubit can only have 0 or 1 bits of entropy, which, for the single reference qubit probe, increases the statistical fluctuations and may lead to stronger finite-size effects in the purification dynamics near $p_c$. Our focus on a single-reference qubit in this work was primarily due to the simplicity of the experimental and numerical implementations, we have not been able to conclusively resolve whether one or several reference qubits are preferable for obtaining accurate critical properties.

Our results for one and four reference qubits maximally entangled with a contiguous region of the system that is otherwise in a product state are shown in Fig. S2(a)-(b). We run the circuit at $p = 0.1596 \approx p_c$ and assume a scaling function of the form

$$\langle S(\rho)\rangle = t^{-\eta_\parallel/2} F(t/L). \quad \text{(S1)}$$

Similar to Li *et al.*, we find that the estimated value of $\eta_\parallel$ with this method drifts to larger values as the size of the

reference system increases (we find $\eta_{||} = 0.70(2)/0.76(2)$ for one/four reference qubits). Our estimated value of $\eta_{||}$ differs slightly from theirs ($\eta_{||} = 0.82$) because we use a slightly smaller estimate for $p_c$ of 0.1596 compared to their estimate of 0.1600. However, all the values reported for $\eta_{||}$ lie within the systematic uncertainty we estimated from the mutual information probes $\eta_{||} = 0.7(1)$. As a result, we leave it to future work to obtain a more accurate estimate of $\eta_{||}$ for this model.

[1] Y. Li, X. Chen, and M. P. A. Fisher, *Measurement-driven entanglement transition in hybrid quantum circuits*, Phys. Rev. B **100**, 134306 (2019).

[2] M. J. Gullans and D. A. Huse, *Dynamical purification phase transition induced by quantum measurements* (2019), arXiv:1905.05195.

[3] Y. Li, X. Chen, A. W. W. Ludwig, and M. P. A. Fisher, *Conformal invariance and quantum non-locality in hybrid quantum circuits* (2020), arXiv:2003.12721.

[4] M. Ippoliti, M. J. Gullans, S. Gopalakrishnan, D. A. Huse, and V. Khemani, *Entanglement phase transitions in measurement-only dynamics* (2020), arXiv:2004.09560.
